# Supplementary material for: Combinatorial Optimization of AC Optimal Power Flow with Discrete Demands in Radial Networks
Source: arXiv:1709.08431 source file (2019-10-15)
Supplement: Supplementary file 1 [file appendix.tex]

%\newpage
\vspace*{-10pt}
\appendix
\vspace*{-5pt}
\subsection{Tree Formulation for OPF}\label{sec:TF}

For convenience, we give another formulation of OPF, based the recursive ``unfolding'' of  Eqns.~\raf{p1:con2}-\raf{p1:con4}. We  start with the following simple lemma.
\begin{lemma}\label{lem:simple}
	Let $F \triangleq \big(s_0,s, v, \ell, S\big)$ be 	a vector satisfying \raf{p1:con2}-\raf{p1:con4}. Then 
	\begin{align}
	&S_{i,j}=\sum_{k \in \cN_j}  s_k + \sum_{e \in \cE_j\cup\{(i,j)\}}z_e \ell_{e}, ~\forall (i,j) \in \cE.\label{TF:S}\\
	&v_j=v_0 -2 \sum_{k \in \cN} \re\Big( \sum_{(h,t)\in \cP_k \cap \cP_j} z^*_{h,t}   s_k \Big) - \nonumber\\ 
	&~~\Big(2 \sum_{(h,t)\in \cP_j} \re \big( z_{h,t}^* \sum_{e \in \cE_t} z_{e}  \ell_{e}\big) +    \sum_{ (h,t) \in\cP_{j} }|z_{h,t}|^2  \ell_{h,t}\Big),~\forall j \in\cV^+. \label{TF:v}
	\end{align}
\end{lemma}
\begin{proof}
	The first  equation is obtained by rewriting  $S_{i,j}$, recursively using Eq.~\raf{p1:con2}, substituting from the leaves. To see the second equation, rewrite Cons.~\raf{p1:con4}  by recursively substituting $v_j$, for $j$, moving away from the root, and then substituting for $S_{h,t}$ using \raf{TF:S}:
	\begin{align}
	v_j &= v_0 -2\sum_{ (h,t) \in \cP_{j} } \re(z_{h,t}^\ast   S_{h,t}) +  \sum_{( h,t) \in \cP_{j} } |z_{h,t}|^2  \ell_{h,t}\notag\\
	&=v_0 -2 \sum_{ (h,t) \in \cP_{j} } \re\Big(z^*_{h,t}\big(\sum_{k\in \cN_t}  s_k + \sum_{e \in \cE_t\cup\{(h,t)\}} z_{e}  \ell_{e} \big)\Big) \notag \\ 
	&~~~ +   \sum_{ (h,t) \in \cP_{j} } |z_{h,t}|^2  \ell_{h,t},\notag\\
	&=v_0 -2 \sum_{k \in \cN} \re\Big( \sum_{(h,t)\in \cP_k \cap \cP_j} z^*_{h,t}   s_k \Big) \notag\\
	&~~~  - 2 \sum_{(h,t)\in \cP_j} \re \Big( z_{h,t}^* \sum_{e \in \cE_t} z_{e}  \ell_{e}\Big)  \notag \\ 
	&~~-    2\sum_{ (h,t) \in\cP_{j} }|z_{h,t}|^2  \ell_{h,t} +\sum_{ (h,t) \in\cP_{j} }|z_{h,t}|^2  \ell_{h,t},  \label{eqn:ch3:vLL}
	\end{align}
	where the last statement follows from exchanging the summation operators, and using $z^*_{e} z_{e} = |z_{e}|^2$. 
\end{proof}

It follows from Lemma~\ref{lem:simple}, that we may equivalently formulate  {\sc OPF} as
\begin{align}
\textsc{(tOPF)}  \ &\min_{\substack{s_0, s, v,\ell, S \;\;}} f(s_0, s),  \notag \\
\text{subject to} \ &\raf{p1:con1},\raf{TF:S},\raf{p1:con3},\raf{TF:v},\raf{p1:con5}-\raf{p1:con9}.\notag 
\end{align}

We shall refer to this as the {\em tree formulation} of  {\sc OPF}. 

\begin{lemma}\label{lem:equiv}
	Formulations {\sc OPF} and {\sc tOPF} are equivalent.
\end{lemma}
\begin{proof}
	Given a feasible solution $F \triangleq \big(s_0,s, v, \ell, S\big)$ of {\sc OPF}, Lemma~\ref{lem:simple} shows that $F$ is also feasible for {\sc tOPF}. Conversely, let $F \triangleq \big(s_0,s, v, \ell, S\big)$ be a feasible solution of {\sc tOPF}, we show by that $F$ satisfies \raf{p1:con2} and \raf{p1:con4}. Consider first~\raf{p1:con2}. Note by~\raf{TF:S} that, for $(i,j)\in\cE$,
	\vspace*{-10pt}
	\begin{align*} 
	S_{i,j}- \sum_{l:(j,l)\in \cE} S_{j,l} &=
	\sum_{k \in \cN_j}  s_k + \sum_{e \in \cE_j\cup\{(i,j)\}}z_e \ell_{e}\\
	&\quad -\left(\sum_{l:(j,l)\in \cE} \sum_{k \in \cN_l}  s_k + \sum_{e \in \cE_l\cup\{(j,l)\}}z_e \ell_{e}\right)\\
	&=\sum_{k \in \cU_j} s_k +z_{i,j}\ell_{i,j}.
	\end{align*}
	Consider next~\raf{p1:con4}. Then~\raf{TF:v} implies that, for $(i,j)\in\cE$, 
	\begin{align*}
	&v_j-v_i=2 \sum_{k \in \cN} \re\Big( \sum_{(h,t)\in \cP_k \cap \cP_i} z^*_{h,t}   s_k\Big) \\
	&\quad -2 \sum_{k \in \cN} \re\Big( \sum_{(h,t)\in \cP_k \cap \cP_j} z^*_{h,t} \Big)  s_k \\
	&\quad +\Big(2 \sum_{(h,t)\in \cP_i} \re \big( z_{h,t}^* \sum_{e \in \cE_t} z_{e}  \ell_{e}\big) +    \sum_{ (h,t) \in\cP_{i} }|z_{h,t}|^2  \ell_{h,t}\Big)\\
	&\quad - \Big(2 \sum_{(h,t)\in \cP_j} \re \big( z_{h,t}^* \sum_{e \in \cE_t} z_{e}  \ell_{e}\big) +    \sum_{ (h,t) \in\cP_{j} }|z_{h,t}|^2  \ell_{h,t}\Big)
	\end{align*}
	\begin{align*}
	&=-2\sum_{k \in \cN_j} \re\Big( \sum_{(h,t)\in \cP_k \cap (\cP_j\setminus \cP_i)} z^*_{h,t} s_k \Big)\\
	&\quad -\Big(2 \sum_{(h,t)\in \cP_j\setminus \cP_i} \re \big( z_{h,t}^* \sum_{e \in \cE_t} z_{e}  \ell_{e}\big) +    \sum_{ (h,t) \in\cP_{j}\setminus \cP_i }|z_{h,t}|^2  \ell_{h,t}\Big)\\
	&=-2\sum_{k \in \cN_j} \re(z^*_{i,j}s_k) -\Big(2 \re \big( z_{i,j}^* \sum_{e \in \cE_j} z_{e}  \ell_{e}\big) +    |z_{i,j}|^2  \ell_{i,j}\Big)\\
	&=-2\sum_{k \in \cN_j} \re(z^*_{i,j}s_k) -2\Big( \re \big( z_{i,j}^* \sum_{e \in \cE_j\cup\{(i,j)\}} z_{e}  \ell_{e}\big) \Big)+    |z_{i,j}|^2  \ell_{i,j}\\
	&=-2\re\Big(z^*_{i,j}\big(\sum_{k \in \cN_j} s_k+\sum_{e \in \cE_j\cup\{(i,j)\}} z_{e}  \ell_{e}\big)\Big)+    |z_{i,j}|^2  \ell_{i,j}\\
	&=-2\re\big( z^*_{i,j}S_{i,j}\big)+    |z_{i,j}|^2  \ell_{i,j}.
	\end{align*}
	where the last equality follows from \raf{TF:S}.
\end{proof}

\vspace*{-10pt}
\subsection{Proof of Theorem~\ref{thm:exact}}
In proving the sufficient condition for exactness of the SOCP relaxation of OPF, we will make use of the following lemma.

\begin{lemma}\label{lem:triv1}
	Let $F \triangleq \big(s_0,s, v, \ell, S\big) $ and $F' \triangleq \big(s_0',s', v', \ell', S'\big) $ be two vectors satisfying \raf{p1:con2}  (or equivalently~\raf{TF:S}), such that $s= s'$ and $\ell\le\ell'$ (component wise). {\color{blue} Suppose also that $F$ satisfies {\sf C2}.} Then under assumption {\sf A1}, $S_{i,j}\le S_{i,j}'$ and $|S_{i,j}|\le|S_{i,j}'|$ for all $(i,j)\in\cE$, and $v_j\ge v_j'$ for all $j\in\cV^+$.  
\end{lemma} 	
\begin{proof}
	Write $\Delta \ell_e \triangleq \ell_e - \ell_e'\le 0$, $\Delta S_e \triangleq  S_e - S_e'$, and $\Delta |S_e|^2 \triangleq  | S_e|^2 - |S_e'|^2$, for  $e\in \cE$. Let $S_{j} \triangleq  \sum_{k \in \cN_j} s_k$,  $ L_{i,j} \triangleq \sum_{e \in \cE_j\cup\{(i,j)\}}z_e \ell_e$, and $ L'_{i,j} \triangleq \sum_{e \in \cE_j\cup\{(i,j)\}}z_e  \ell_e'$. Note by \raf{TF:S} that $\tilde S_{i,j} = S_{j} +  L_{i,j}$ and,  similarly, $ S_{i,j}' =  S_{j} +  L_{i,j}'$. It follows that, for all $(i,j)\in\cE$,
	\begin{align}\label{eqn:ch3:lem1.0--}
	\Delta S_{i,j} &=   L_{i,j}-L_{i,j}'=\sum_{e \in \cE_j\cup\{(i,j)\}}z_{e} \Delta \ell_{e} \le 0,
	\end{align}
	where the inequality follows by assumption {\sf A1}. This implies that $S_{i,j}\le S_{i,j}'$.	
	Furthermore,
	\begin{align}
	&\Delta |S_{i,j}|^2 = | S_{i,j}|^2 - |S_{i,j}'|^2\\
	&~= ( S_{i,j}^{\rm R})^2 -  (S_{i,j}'^{\rm R})^2 +( S_{i,j}^{\rm I})^2 - (S_{i,j}'^{\rm I})^2 \\
	&~=\Delta S_{i,j}^{\rm R} ( S_{i,j}^{\rm R} +  S_{i,j}'^{\rm R}) + \Delta S_{i,j}^{\rm I} ( S_{i,j}^{\rm I} +  S_{i,j}'^{\rm I})\\
	&~=\sum_{e \in \cE_j\cup\{(i,j)\}} z_e^{\rm R} \Delta \ell_e \big( 2  S^{\rm R}_{j} +  L_{i,j}^{\rm R} + L_{i,j}'^{\rm R} \big)\nonumber\\
	&\quad+ \sum_{e \in \cE_j\cup\{(i,j)\}} z_e^{\rm I} \Delta \ell_e \big( 2  S^{\rm I}_{j} +  L_{i,j}^{\rm I} + L_{i,j}'^{\rm I} \big) \\
	&~= \sum_{e \in \cE_j\cup\{(i,j)\}}  2\Delta \ell_e \re(z_e^* S_j)+ \sum_{e \in \cE_j\cup\{(i,j)\}}  \Delta \ell_e \re(z_e^* L_{i,j})\nonumber\\&\quad +\sum_{e \in \cE_j\cup\{(i,j)\}}  \Delta \ell_e\re(z_e^*L'_{i,j})\le 0,
	\end{align}
	where the Inequality follows by {\sf A1}, {\sf C2} and $\Delta \ell_e \le 0$. Therefore
	$|S_{i,j}|\le|S_{i,j}'|$.
	Finally, using~\raf{TF:v}, we get by {\sf A1} that
	\begin{align*}
	 v_j-v_j'&= - \Big(2 \sum_{(h,t)\in \cP_j} \re \big( z_{h,t}^*\sum_{e \in \cE_t} z_{e}  \Delta\ell_{e}\big) \\
	 &\qquad~~ +    \sum_{ (h,t) \in\cP_{j} }|z_{h,t}|^2  \Delta\ell_{h,t}\Big)\ge 0.
	\end{align*}	
	 
\end{proof}

\begin{corollary}\label{lem:triv}
	Let $F \triangleq \big(s_0,s, v, \ell, S\big) $ be	a vector satisfying \raf{p1:con2}, \raf{p1:con3} and \raf{p1:con4} (or equivalently\raf{TF:S}, \raf{p1:con3} and \raf{TF:v}), and $|S_{i,j}| \le \overline S_{i.j},$ for all $(i,j)\in\cE$. {\color{blue} Suppose also that $F$ satisfies {\sf C2}.} Then under assumptions {\sf A1}   and {\sf A2}, $F$ also satisfies $v_j \le \overline v_j $, for all $j\in\cV^+$, and $|S_{i,j}- z_{i,j}\ell_{i,j}| \le \overline S_{i,j}$, for all $(i,j)\in\cE$. 
\end{corollary}
\begin{proof}
	The first claim is immediate from ~\raf{TF:v} and assumptions {\sf A1},   {\sf A2}  and  {\sf C2} as
	\begin{align*}
	v_j&=v_0 -2 \sum_{(h,t)\in \cP_j}\sum_{k \in \cN_t} \re\big( z^*_{h,t}  s_k \big) - \nonumber\\ 
	&\quad\Big(2 \sum_{(h,t)\in \cP_j} \re \big( z_{h,t}^* \sum_{e \in \cE_t} z_{e}  \ell_{e}\big) +    \sum_{ (h,t) \in\cP_{j} }|z_{h,t}|^2  \ell_{h,t}\Big).
	\end{align*}
	The second claim follows from Lemma~\ref{lem:triv1} as $F'\triangleq \big(s_0,s, v, \ell', S'\big)$ with 
	\begin{align*}
	\ell'_{t,h}&\triangleq\left\{\begin{array}{ll}
	0&\text{ if }(t,h)=(i,j) \\
	\ell_{t,h}&\text{ otherwise, } 
	\end{array}
	\right.
	\end{align*}
	satisfies $S_{i,j}'=S_{i,j}- z_{i,j}\ell_{i,j}$.
\end{proof}

\vspace*{-10pt}
\begin{customthm}{\ref{thm:exact}} Let $F''=(s_0'', s', v',\ell'',S'')$ be a feasible solution of {\sc cOPF}$[s']$  {\color{blue} satisfying {\sf C2}}. Under assumptions~{\sf A0}, {\sf A1}, and {\sf A2}, there a feasible solution  $F'=(s_0', s', v',\ell',S')$ of {\sc cOPF}$[s']$ that satisfies  $\ell'_{i,j} = \frac{|S_{i,j}'|^2}{v_i'}$ for all  $(i,j)\in \cE,$ and $f(F')\le f(F'')$. Given $F''$, such a solution $F'$ can be found in polynomial time.  
\end{customthm}

\begin{IEEEproof}
	The proof follows essentially the same lines as in \cite{gan2015exact, low2014convex1, low2014convex2,huang2017sufficient}. 
	We consider the following convex program\footnote{Typical convex programming solvers return a solution that is feasible within an absolute error $\epsilon>0$, where the running time depends on $\log\frac{1}{\epsilon}$. For simplicity, we assume that the convex program can be solved exactly.}: 
	\begin{align}
	\textsc{(cOPF$'[s']$)}  \ &\min_{\substack{s_0, s, v,\ell, S \;\;}}\sum_{e\in\cE}\ell_e,  \notag \\
	\text{subject to} \ &\raf{p1:con2}-\raf{p1:con5}, \raf{p1:con9}, \raf{p2:con1}\notag \\
	& \ell_{i,j} \le \ell_{i,j}'',  ~~\forall (i,j) \in \cE \label{p3:con7}\\
	& s_k = s'_k,~~\forall k \in \cN. \label{p3:con8} 
	\end{align}
	Clearly,  \textsc{cOPF$'[s']$}  is feasible as $F''$ satisfies all its constraints. Hence, it has an optimal solution $F'=(s_0', s', v',\ell',S')$, which we claim to satisfy the statement of the theorem.  First, we observe that $F'$ is an optimal solution for {\sc cOPF}$[s']$ (minimizing $\sum_{e\in\cE}\ell_e$ among all such solutions). Indeed, Ineq. \raf{p3:con7} implies that
	\begin{align}\label{e-l-}
	\ell_e' \le \ell_e''\le \overline \ell_e\text{ for all  $e \in \cE$.}
	\end{align}
	It follows by Lemma~\ref{lem:triv1} and the feasibility of $F''$ for {\sc cOPF}$[s']$  that, for all $(i,j)\in\cE$,
	\begin{align}\label{eqn:ch3:lem1.0}
	S_{i,j}' \le S_{i,j}''\text{ and } |S_{i,j}'| \le |S_{i,j}''| \le \overline S_{i,j} .
	\end{align}
	In particular, for $(i,j)=(0,1)$, we obtain 
	\begin{align}\label{s-e}
	-s_0'^{\rm R} &=  S_{0,1}'^{\rm R}  \le S_{0,1}''^{\rm R} = -s_0''^{\rm R},
	\end{align}
	implying by {\sf A0} that $f_0( -s_0'^{\rm R})  \le f_0(-s_0''^{\rm R})$ and hence by \raf{p3:con8}, $f(s_0',s')\le f(s_0'',s')$.
	
	Note also that, since $F'$ satisfies ~\raf{p1:con2}-\raf{p1:con4}, we have by Corollary~\ref{lem:triv} that $|S_{i,j}'- z_{i,j}\ell_{i,j}'| \le \overline S_{i,j}$, for all $(i,j)\in\cE$. We conclude the feasibility of $F'$ for {\sc cOPF}$[s']$.
	
	Next, suppose, for the sake of contradiction, that there exists an edge $(h,t)$ such that $\ell_{h,t}' > \tfrac{|S_{h,t}'|^2}{v'_h}$.
	We  construct a feasible solution $\tilde F=(\tilde s_0, s', \tilde v, \tilde \ell, \tilde S)$ for \textsc{cOPF$'[s']$} such that  $\sum_{e\in\cE}\tilde\ell_e<\sum_{e\in\cE}\ell_e'$, leading to a contradiction to the optimality of $F'$ for {\sc cOPF}$'[s']$.
	
	To obtain $\tilde F=(\tilde s_0,s',\tilde v,\tilde \ell, \tilde S)$ from $F'$, we set  $\tilde \ell_{i,j} \leftarrow \frac{|S_{i,j}'|^2}{v_i'}$, then obtain $\tilde S$ and $\tilde v$ by substituting $\ell\leftarrow\tilde\ell$ in Eqns.~\raf{TF:S} and~\raf{TF:v}. To complete the proof, we show the feasibility of $\tilde F$.
	
	By the way we constructed $\tilde F$, all equality constraints of \textsc{cOPF$'[s']$}  are satisfied (via Lemma~\ref{lem:equiv}), and
	by the feasibility of $F'$ for {\sc cOPF}$[s']$ (in particular, Ineq.~\raf{p2:con1}), we also have 
	\begin{align}\label{e-l}
	\tilde \ell_{i,j}=\frac{|S_{i,j}'|^2}{v_i'} \le \ell_{i,j}'\le \ell_{i,j}''\text{ for all  $(i,j) \in \cE$.}
	\end{align}
	It follows by Lemma~\ref{lem:triv1} and the feasibility of $F'$ that
	\begin{align}\label{eqn:ch3:lem1.0-}
	\tilde S_{i,j} \le S_{i,j}'\text{ and } |\tilde S_{i,j}| \le |S_{i,j}'|,~~, \forall (i,j)\in\cE,\\
	\tilde v_j\ge v_j'\ge\underline v_j,~~\forall j\in\cV^+.\label{eqn:ch3:lem1.1-}
	\end{align}
	Note also that, since $\tilde F$ satisfies ~\raf{p1:con2}-\raf{p1:con4} {\color{blue}and {\sf C2}}, we have by Corollary~\ref{lem:triv} that $\tilde v_j\le\overline{v}_j$ for all $j\in\cV^+$.
	Moreover, by Ineqs.~\raf{eqn:ch3:lem1.0-} and \raf{eqn:ch3:lem1.1-}, $\tilde \ell_{i,j} = \frac{| S_{i,j} '|^2}{v_i'} \ge \frac{| \tilde S_{i,j} |^2}{\tilde v_i}$, hence, $\tilde F$ is feasible for \textsc{cOPF$'[s']$}.
	
	Finally by the first inequality in \raf{e-l} and the fact that $\ell_{h,t} '> \tfrac{|S_{h,t}|^2}{v_h}=\tilde\ell_{h,t} $, we have $\sum_{e\in\cE}\tilde \ell_{e}<\sum_{e\in\cE} \ell_{e}'$, contradicting the optimality of $F'$ for \textsc{cOPF$'[s']$}.
\end{IEEEproof}

%\begin{theorem}
%There is a bijection between {\sc OPF$^\phi$} and {\sc OPF}. 
%Also, there is a bijection between {\sc cOPF$^\phi$} and {\sc cOPF}.		
%\end{theorem}
%
%\begin{IEEEproof}
%A feasible solution $F=(s_0,s,S,v,\ell)$ of  {\sc OPF$^\phi$} can be mapped to a feasible solution ${\tilde F}=({\tilde s}_0, {\tilde s},{\tilde S},v,\ell)$ of OPF, where ${\tilde S}_{i,j}\triangleq S_{i,j} e^{-{\bf i}\phi}, {\tilde s}_0\triangleq s_0 e^{-{\bf i} \phi}$, and vise versa. Similarly, it holds for {\sc cOPF$^\phi$} and {\sc cOPF}.
%\end{IEEEproof}

\subsection{Additional Information of Evaluation Studies}
{\color{blue} The single-line diagram and line data of the RBTS 13-node  network are presented in Fig.~\ref{fig:net} and Table~\ref{tab:net}, respectively.

\begin{figure}[!htb]\vspace{-10pt}
	\begin{center}
		\includegraphics[scale=.7]{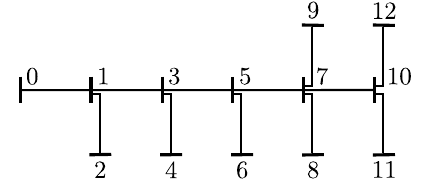}
	\end{center}%\vspace{-5pt}
	\caption{Single-line diagram of the RBTS 13-node electric network.}
	\label{fig:net}
\end{figure} 

\begin{table}[!htb]
	%  1 is the default, change whatever you need 
	\centering 
	{\scriptsize 
		\begin{tabular}{c|l|l|l} 
			\hline
			\hline \vspace{-5pt}   Bus  & \hfill R \hfill  & \hfill X  \hfill   & \hfill Capacity \hfill \\ 
			& \hfill (p.u.) \hfill  &   \hfill(p.u.)\hfill  & \hfill(p.u.)\hfill\\ 
			\hline
			\hline $(0 , 1)$ &  $0.011636363636364$ & $0.034380165289256$ & $1$\\
			\hline $(1 , 2)$ &  $0.026446280991736$ & $0.158677685950413$ & $0.125$\\
			\hline $(1 , 3)$ &  $0.014545454545455$ & $0.043636363636364$ & $0.7625$\\
			\hline $(3 , 4)$ &  $0.026446280991736$ & $0.158677685950413$ & $0.25$\\
			\hline $(3 , 5)$ &  $0.017454545454546$ & $0.042314049586777$ & $0.75$\\
			\hline $(5 , 6)$ &  $0.026446280991736$ & $0.158677685950413$ & $0.25$\\
			\hline $(5 , 7)$ &  $0.011636363636364$ & $0.03702479338843 $ & $0.75$\\
			\hline $(7 , 8)$ &  $0.026446280991736$ & $0.171900826446281$ & $0.25$\\
			\hline $(7 , 9)$ &  $0.031735537190083$ & $0.185123966942149$ & $0.25$\\
			\hline $(7 , 10)$&  $0.014545454545455$ & $0.039669421487603$ & $0.75$\\
			\hline $(10, 11)$&  $0.013223140495868$ & $0.161322314049587$ & $0.25$\\
			\hline $(10, 12)$&  $0.029090909090909$ & $0.185123966942149$ & $0.25$\\
			\hline \hline
		\end{tabular}  
	} 
	\caption{Settings of line impedance and maximum capacity of the RBTS 13-node electric network.} 
	\label{tab:net} 
\end{table} 
%A linear objective function is considered in the simulations, which is defined as:
%\begin{equation}
%f'(x) \triangleq \sum_{k \in \cI} \overline f_k (1-x_k) %+ \sum_{e \in \cE} z_e^{\rm R} \ell_e.
%\end{equation}
%One can easily show that $f'$ is a special case of the objective function $f$ (Eqn.~\raf{eq:obj}). $\overline f_k$ is the penalty (or cost) of  not satisfying demand $s_k$.

The simulations were evaluated using Intel i7-3770 CPU $3.40$GHz processor with $32$GB of RAM. The algorithms were implemented using Python 2.7 programming language with Scipy library for scientific computation. }

%The IEEE 123-node network is unbalanced three-phase networks with several devices that are not modeled in {\sc OPF}. As in \cite{gan2015exact}, one can modify the IEEE network by the following:
%\begin{itemize}
%	\item The three phases are assumed to be decoupled into three identical single phase networks.
%	\item Closed circuit switches are modeled as shorted lines and ignore open circuit switches.
%	\item Transformers are modeled as lines with appropriate impedances.
%\end{itemize}
